# Supplementary material for: Wavelet-Packets for Deepfake Image Analysis and Detection
Source: arXiv:2106.09369 source file (2022-09-01)
Supplement: Supplementary file 1 [file db5.tex]

\documentclass{standalone}
\usepackage[utf8]{inputenc}
\usepackage{pgfplots}
\DeclareUnicodeCharacter{2212}{−}
\usepgfplotslibrary{groupplots,dateplot}
\usetikzlibrary{patterns,shapes.arrows}
\pgfplotsset{compat=newest}
\begin{document}
% This file was created by tikzplotlib v0.9.8.
\begin{tikzpicture}

\definecolor{color0}{rgb}{0.12156862745098,0.466666666666667,0.705882352941177}
\definecolor{color1}{rgb}{1,0.498039215686275,0.0549019607843137}
\definecolor{color2}{rgb}{0.172549019607843,0.627450980392157,0.172549019607843}
\definecolor{color3}{rgb}{0.83921568627451,0.152941176470588,0.156862745098039}

\begin{axis}[
legend cell align={left},
legend style={
  fill opacity=0.8,
  draw opacity=1,
  text opacity=1,
  at={(0.03,0.03)},
  anchor=south west,
  draw=white!80!black
},
tick align=outside,
tick pos=left,
title={Daubechies 5},
x grid style={white!69.0196078431373!black},
xmin=0.45, xmax=10.45,
xtick style={color=black},
y grid style={white!69.0196078431373!black},
ymin=-0.79673938128155, ymax=0.79673938128155,
ytick style={color=black}
]
\addplot [densely dashed, mark=triangle, mark size=3, mark options={solid}, color0]
table {%
1 0.00333572528547377
2 -0.012580751999082
3 -0.00624149021279827
4 0.0775714938400457
5 -0.0322448695846384
6 -0.242294887066382
7 0.138428145901321
8 0.724308528437773
9 0.60382926979719
10 0.160102397974193
};
\addlegendentry{$\mathbf{h}_\mathcal{L}$}
\addplot [solid, mark=o, mark size=3, mark options={solid}, color1]
table {%
1 -0.160102397974193
2 0.60382926979719
3 -0.724308528437773
4 0.138428145901321
5 0.242294887066382
6 -0.0322448695846384
7 -0.0775714938400457
8 -0.00624149021279827
9 0.012580751999082
10 0.00333572528547377
};
\addlegendentry{$\mathbf{h}_\mathcal{H}$}
\addplot [solid, mark=o, mark size=3, mark options={solid}, color2]
table {%
1 0.160102397974193
2 0.60382926979719
3 0.724308528437773
4 0.138428145901321
5 -0.242294887066382
6 -0.0322448695846384
7 0.0775714938400457
8 -0.00624149021279827
9 -0.012580751999082
10 0.00333572528547377
};
\addlegendentry{$\mathbf{f}_\mathcal{L}$}
\addplot [densely dashed, mark=triangle, mark size=3, mark options={solid}, color3]
table {%
1 0.00333572528547377
2 0.012580751999082
3 -0.00624149021279827
4 -0.0775714938400457
5 -0.0322448695846384
6 0.242294887066382
7 0.138428145901321
8 -0.724308528437773
9 0.60382926979719
10 -0.160102397974193
};
\addlegendentry{$\mathbf{f}_\mathcal{H}$}
\end{axis}

\end{tikzpicture}

\end{document}
