# Supplementary material for: Wavelet-Packets for Deepfake Image Analysis and Detection
Source: arXiv:2106.09369 source file (2022-09-01)
Supplement: Supplementary file 6 [file lsun_packet_mean_std_plot.tex]

\documentclass{standalone}
\usepackage[utf8]{inputenc}
\usepackage{pgfplots}
\DeclareUnicodeCharacter{2212}{−}
\usepgfplotslibrary{groupplots,dateplot}
\usetikzlibrary{patterns,shapes.arrows}
\pgfplotsset{compat=newest}
\begin{document}
% This file was created by tikzplotlib v0.9.8.
% [inline block 0: 1 envs, 66625 chars -> data_tex | \begin{tikzpicture} ...]


\end{document}
