# Supplementary material for: Wavelet-Packets for Deepfake Image Analysis and Detection
Source: arXiv:2106.09369 source file (2022-09-01)
Supplement: Supplementary file 14 [file synthesis_haar_level_2.tex]

\documentclass{standalone}
\usepackage[utf8]{inputenc}
\usepackage{pgfplots}
\DeclareUnicodeCharacter{2212}{−}
\usepgfplotslibrary{groupplots,dateplot}
\usetikzlibrary{patterns,shapes.arrows}
\pgfplotsset{compat=newest}
\pgfplotsset{ticks=none}
\begin{document}
% This file was created by tikzplotlib v0.9.8.
\begin{tikzpicture}

\begin{axis}[
tick align=outside,
tick pos=left,
title={synthesis haar level 2.tex},
x grid style={white!69.0196078431373!black},
xmin=-0.5, xmax=575.5,
xtick style={color=black},
y dir=reverse,
y grid style={white!69.0196078431373!black},
ymin=-0.5, ymax=575.5,
ytick style={color=black}
]
\addplot graphics [includegraphics cmd=\pgfimage,xmin=-0.5, xmax=575.5, ymin=575.5, ymax=-0.5] {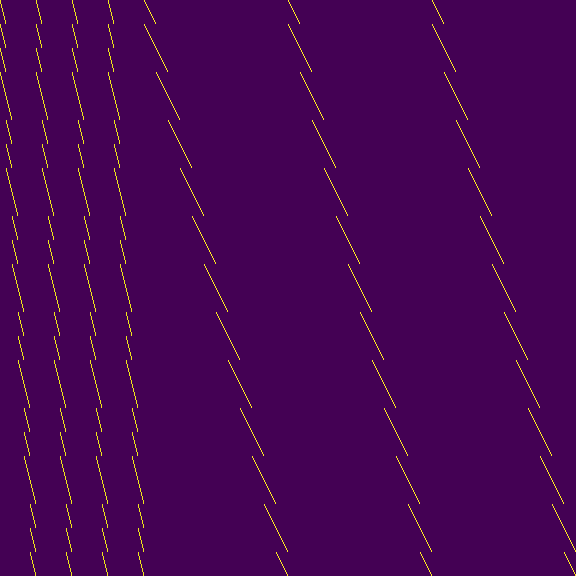};
\end{axis}

\end{tikzpicture}

\end{document}
